# Supplementary material for: On the Possibility of Melting Water Ice during the Recent Past of Mars: Application to the Formation of Gullies
Source: arXiv:2510.06154 source file (2026-01-08)
Supplement: Supplementary file 1 [file Lange_Forget_supp.pdf]

**On the Possibility of Melting Water Ice during the Recent Past of Mars.  
Application to the Formation of Gullies.**

Lange, L.<sup>1</sup> & Forget, F.<sup>1</sup>

<sup>1</sup> Laboratoire de Météorologie Dynamique, Institut Pierre-Simon Laplace (LMD/IPSL),  
Sorbonne Université, Centre National de la Recherche Scientifique (CNRS), École  
Polytechnique, École Normale Supérieure (ENS), Paris, France

**Contents of this file**

Text S1 to S4

Figures S1 to S4

Table S1

**Introduction**

This supporting document is composed of three sections detailing the model used and the model validation, four supporting figures, and one supporting table.

- The first section describes the modeling of the water vapor seasonal cycle in the 1D model and is associated with Figure S1 validating the design of our implementation.
- The second section describes the sublimation model used in this study, along with comparisons with Earth in-situ measurements of sublimation presented in Figure S2.
- The third section demonstrates the formulation used to compute subsurface ice sublimation flux.
- The fourth section explains how we estimate the amount of liquid water generated by the melting of subsurface ice.
- Figure S3 shows the dependence of the maximum subsurface ice temperature with depth.
- Figure S4 shows the amount of liquid water formed by the sublimation of subsurface ice (in unrealistic conditions) during a few Martian sols in summer.
- Table S1 describes the set-up for the simulations performed in section 3.3

### Text S1: Modeling the diurnal and seasonal variations of water vapor in the 1D model

The lateral transport of water in the atmosphere is represented in the 1D model with a nudging toward a mean value. The mixing ratio of water vapor  $q_{\text{vap}}$  ( $\text{kg kg}^{-1}$ ) given as input to the physics input at time  $t + \Delta t$  (s) is:

$$q_{\text{vap}}(t + \Delta t) = \underbrace{\frac{m_{\text{H}_2\text{O}} \times g}{P_{\text{surf}}}}_{\text{average mass mixing ratio of H}_2\text{O in the column}} + \left( q_{\text{vap,model}}(t + \Delta t) - \frac{m_{\text{H}_2\text{O}} \times g}{P_{\text{surf}}} \right) e^{-\frac{\Delta t}{\tau}}$$

where  $m_{\text{H}_2\text{O}}$  ( $\text{kg m}^{-2}$ ) is the nudging value of the  $\text{H}_2\text{O}$  mass in the column per unit area,  $q_{\text{vap,model}}(t + \Delta t)$  is the value of the water vapor mixing ratio predicted by the 1D model at time  $t + \Delta t$  ( $\Delta t$  being the timestep of the model), and  $\tau$  (s) is the relaxation time. We also assume that clouds are advected away from the atmospheric column after each time step, so the mixing ratio of water ice in the air is always set to zero before entering a new time step.

To determine the nudging parameters ( $m_{\text{H}_2\text{O}}$ ,  $\tau$ ), we compared the water vapor in the first atmospheric layer of the model ( $\sim 4$  m) and the amount of water frost on the surface between the 1D model, for several nudging values, and the 3D model (with similar surface conditions - pressure, surface optical/thermophysical properties). An example is given in Figure S1 for latitude  $56.25^\circ\text{N}$  where two values of  $m_{\text{H}_2\text{O}}$  were tested: 15  $\text{pr-}\mu\text{m}$ , the yearly average value measured by TES (Smith, 2002), and 25  $\text{pr-}\mu\text{m}$ , the maximum value measured by TES over the year at this latitude. Comparison with the 3D model shows that it is necessary to use the maximum value over the year measured by TES at a given latitude to better represent the annual water cycle. By testing several values of the relaxation time  $\tau$ , it appears that choosing a relaxation time of 1/2 sol or 1/4 sol (not shown in Figure S1) is optimal.

### Text S2: Modeling the sublimation of water ice at the surface: theory and validation.

The sublimation of water frost/ice on the surface  $F_{\text{ice}}$  ( $\text{kg m}^{-2} \text{s}^{-1}$ ) is given by (Lange et al., 2024):

$$F_{\text{ice}} = C_q U (\rho_{\text{vap,atm}} - \rho_{\text{sv}}(T_{\text{ice}}))$$

where  $C_q$  (unitless) is a moisture transfer coefficient that depends on the stability of the atmosphere (Colaitis et al., 2013, Khuller and Clow, 2024, Lange et al., 2024),  $U$  ( $\text{m s}^{-1}$ ) is the wind velocity obtained by combining the large-scale (synoptic) wind near the surface with a wind gustiness induced by buoyancy (Colaitis et al., 2013),  $\rho_{\text{vap,atm}}$  ( $\text{kg m}^{-3}$ ) the water vapor density in the near-surface layer (altitude  $z_1$  of  $\sim 4$  m),

$\rho_{sv}(T_{ice})$  ( $\text{kg m}^{-3}$ ) the water vapor density at the icy surface derived from the ice temperature  $T_{ice}$  (K) (Murphy & Koop, 2005). The coefficient  $C_q$  is given by:

$$C_q = f_q(Ri) \left( \frac{\kappa^2}{\ln \frac{z_1}{z_0} \ln \frac{z_1}{z_{0q}}} \right)$$

where  $f_q(Ri)$  (unitless) is a function of the Richardson number  $Ri$ ,  $\kappa$  (unitless) is the von Kármán constant set to 0.4;  $z_0$  (m) is the aerodynamic roughness coefficient extracted from Hébrard et al. (2012),  $z_{0q}$  (m) the moisture roughness length derived from the Reynolds and Prandtl numbers (see Eq. 6 of Lange et al. (2024)). The stability functions  $f_q(Ri)$ , given by England and McNider (1995), amplifies the sublimation for an unstable atmosphere, while it reduces it for a stable atmosphere. The Richardson number  $Ri$  is the ratio of the buoyancy term to the flow shear term, and depicts the stability of the atmosphere:

$$Ri = \frac{gz_1}{\theta_{vs}} \frac{(\theta_v(z_1) - \theta_{vs})}{U^2}$$

where  $g$  ( $\text{m s}^{-2}$ ) is the gravity field,  $\theta_{vs}$  (K) is the virtual surface temperature,  $\theta_v(z_1)$  (K) is the virtual temperature at altitude  $z_1$ . This quantity (see expression in Eq. 8 of Lange et al., 2024) represents the temperature that dry air with the same density and pressure as moist air would have.  $Ri = 0$  for a neutral atmosphere,  $Ri < 0$  for an unstable atmosphere,  $Ri > 0$  for a stable atmosphere. Hence, using virtual temperature, the stability of the atmosphere, and thus the sublimation of water ice, is determined by 1) the contrast of density between the near-surface air and atmosphere induced by the difference of temperature and 2) the contrast of density between the moist air at the surface where ice is subliming, and the atmosphere mainly composed of  $\text{CO}_2$ . While the latter effect is included in the Richardson number and the stability function in our model, we do not include it when computing the gustiness' wind. This is left as future work as it would require significant changes in the Planetary Boundary Layer within the Mars PCM.

Our sublimation model is tested against the latent heat-flux measurements on Earth as presented in Khuller and Clow (2024). These measurements were made at several sites: a glacier in the Purcell Mountains in Canada (Fitzpatrick et al., 2017), oceanic surfaces (Fairall et al., 1996; 2003), an ice-covered lake in the Dry Valleys of Antarctica (Clow et al., 1988) and an underground permafrost tunnel in Alaska (Douglas & Mellon, 2019). The same input parameters as those of Khuller & Clow

(2024) are used. The wind used in our model  $U$  is the one provided by measurements and we do not add the gustiness velocity derived in our model (Colaitis et al. (2013)). To quantify the validity of our model, we use the same metrics as them, i.e., the root mean square error (RMSE), and the dimensionless index of agreement ( $d_i$ ) (see their section 5 for definition). Results are shown in Figure S2.

Our model performs reasonably well when modeling the ice sublimation at Purcell Mountains (Figure S2a,  $d_i = 65\%$  in our model, 69% for Khuller & Clow (2024)). As in Khuller & Clow (2024), the main discrepancy between our model and measurements comes from the presence of strong low-level katabatic winds which violates some assumptions of the Monin-Obukhov similarity theory on which our model relies. However, our model does not perform well on smooth ocean surfaces (Figure S2b,  $d_i = 19\%$  vs 62% for Khuller & Clow 2024). The main reasons are: 1) the expression of  $z_{0q}$  we used might not be accurate for such smooth surfaces (e.g., Andreas, 1987); 2) the absence of gustiness velocity in our model (for this comparison only), while it might play a significant role, especially for low-wind periods ("free-convective periods"). Note that such conditions are unlikely on Mars at gully locations because of the presence of strong slope winds (Smith & Spiga, 2018; Spiga & Smith, 2018).

Our model performs very well at Mars Analog sites on Earth. Figure S2c shows that our modeled sublimation rates of ice with the conditions of the dry valleys in Antarctica are in excellent agreement with the ones observed ( $d_i = 92\%$ , similarly to Khuller & Clow (2024)). At the permafrost site in Alaska, for wind velocity of  $0.05 \text{ m s}^{-1}$  to  $0.15 \text{ m s}^{-1}$ , and surface roughness between 10 and 15 cm, our model predicts a sublimation rate between 1.6 cm per year to 2.95 cm per year vs 2.1 cm per year measured. Note that other models, except the one from Khuller & Clow (2024), predicted a sublimation rate 4 times higher than the one measured (Douglas & Mellon 2019).

Hence, our model is validated at Mars Analog sites on Earth and glaciers in Canada, but not on the very smooth oceanic surface, especially during free-convective periods. Given that these conditions are unlikely on Mars at gully sites due to the presence of slope winds, we will consider that our model is reliable for this study, although improvements (especially by adding the effect of water buoyancy on the gustiness) will be considered for future studies.

### **Text S3: Modeling the sublimation of subsurface water ice:**

The determination of the sublimation rate of subsurface ice is made using similar arguments to those presented in Schorghofer (2020). The flux of vapor in the soil

between subsurface ice subliming at depth  $z_{\text{ice}}$  (m) and the surface ( $F_{\text{subsurface ice}}$ ,  $\text{kg m}^{-2} \text{s}^{-1}$ ) is given by (Hudson et al., 2007):

$$F_{\text{subsurface ice}} = \frac{D}{z_{\text{ice}}} \frac{1}{1 - \frac{\rho_{\text{vap,atm}}}{\rho_{\text{sv}}(T_{\text{ice}})}} \left( \rho_{\text{sv}}(T_{\text{ice}}) - \rho_{\text{vap, surf}} \right)$$

where  $D$  ( $\text{m}^2 \text{s}^{-1}$ ) is the diffusion coefficient of the ground, and  $\rho_{\text{vap,surf}}$  ( $\text{kg m}^{-3}$ ) is the water vapor density at the surface.

The flux of water vapor from the surface to the atmosphere  $F_{\text{surf}}$  ( $\text{kg m}^{-2} \text{s}^{-1}$ ) is given by:

$$F_{\text{surf}} = C_q U (\rho_{\text{vap,atm}} - \rho_{\text{vap,surf}})$$

Let's define:

$$R = \frac{C_q U z_{\text{ice}}}{D} \left( 1 - \frac{\rho_{\text{vap,atm}}}{\rho_{\text{sv}}(T_{\text{ice}})} \right)$$

Mass conservation requires that  $F_{\text{subsurface ice}} = F_{\text{surf}}$ . After some development, we get:

$$\rho_{\text{surf}} = \frac{\rho_{\text{sv}}(T_{\text{ice}}) + R \rho_{\text{vap,atm}}}{1 + R}$$

Reinjecting this expression in  $F_{\text{surf}}$  or  $F_{\text{subsurface ice}}$  leads to:

$$F_{\text{ice}} = \frac{D}{z_{\text{ice}}} \frac{1}{1 - \frac{\rho_{\text{vap,atm}}}{\rho_{\text{sv}}(T_{\text{ice}})}} \left( \rho_{\text{sv}}(T_{\text{surf}}) - \rho_{\text{sv}}(T_{\text{ice}}) \right)$$

**Text S4: Estimation of the amount of ice melting:**

We assume that ice melts when the soil-grid mesh has a temperature above 273.15 K. We then look at the grid meshes below which also have a temperature above 273.15 K. The quantity of liquid water generated by this melting is then computed following:

$$m_{\text{H}_2\text{O},\text{liq}} = \int_z \frac{(T_{\text{ice}}(z) - 273.15)}{L_{\text{melt}}} C dz$$

where  $m_{\text{H}_2\text{O},\text{liq}}$  ( $\text{kg m}^{-2}$ ) is the amount of liquid water,  $T_{\text{ice}}$  (K) the ice temperature at depth  $z$  (m),  $L_{\text{melt}}$  the latent heat of fusion set to  $333.55 \text{ kJ kg}^{-1}$ ,  $C$  the water heat capacity set to  $2090 \text{ J kg}^{-1} \text{ K}^{-1}$ . Note that the integration is only performed at depth where  $T_{\text{ice}} > 273.15 \text{ K}$ .

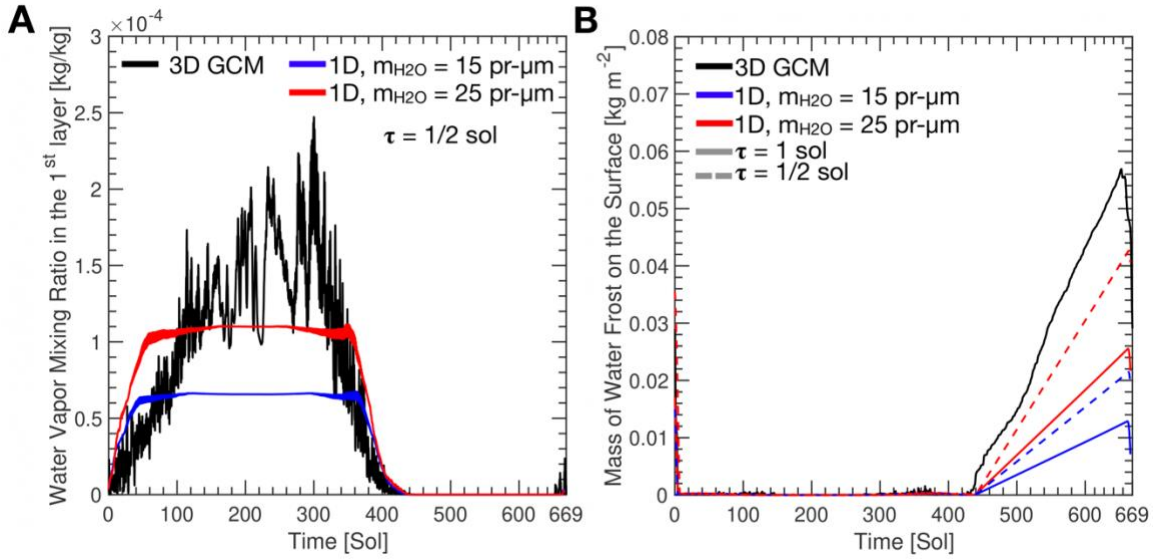

**Figure S1.** a) Mass mixing ratio of the water vapor in the first layer ( $\sim 5$  m) of the model (black curves) at a latitude of  $56.25^\circ\text{N}$  (longitudinally averaged), for  $m_{\text{H}_2\text{O}} = 15$  pr- $\mu\text{m}$  (blue curve) and  $m_{\text{H}_2\text{O}} = 25$  pr- $\mu\text{m}$  (red curve). In these simulations,  $\tau$  is set to half of a Sol duration. b) Frost thickness predicted by the 3D and the 1D, for the same  $m_{\text{H}_2\text{O}}$  as a), and for several relaxation times (one sol for the plain curve, half a sol for the dashed lines).

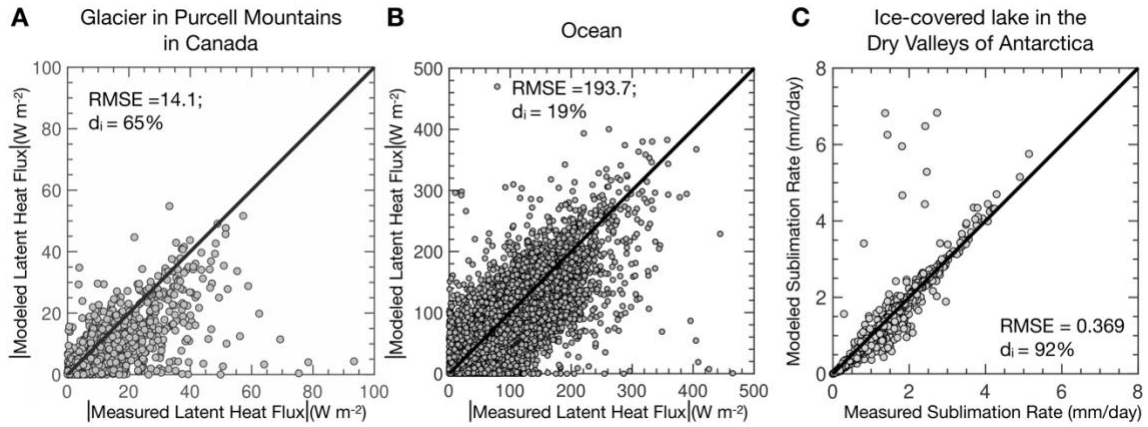

**Figure S2.** a) Comparison between modeled vs measured absolute latent heat flux (a, b) and sublimation rate (c) for a) ice glacier in Purcell Mountains (Fitzpatrick et al., 2017), b) oceanic surfaces (Fairall et al., 1996; 2003), and c) an ice-covered lake in the Dry Valleys of Antarctica (Clow et al., 1988). The black line indicates perfect agreement between measured and modeled values. For each case, the root mean square error and dimensionless index of agreement ( $d_i$ ) (see section 5 of Khuller & Clow (2024)) are given.

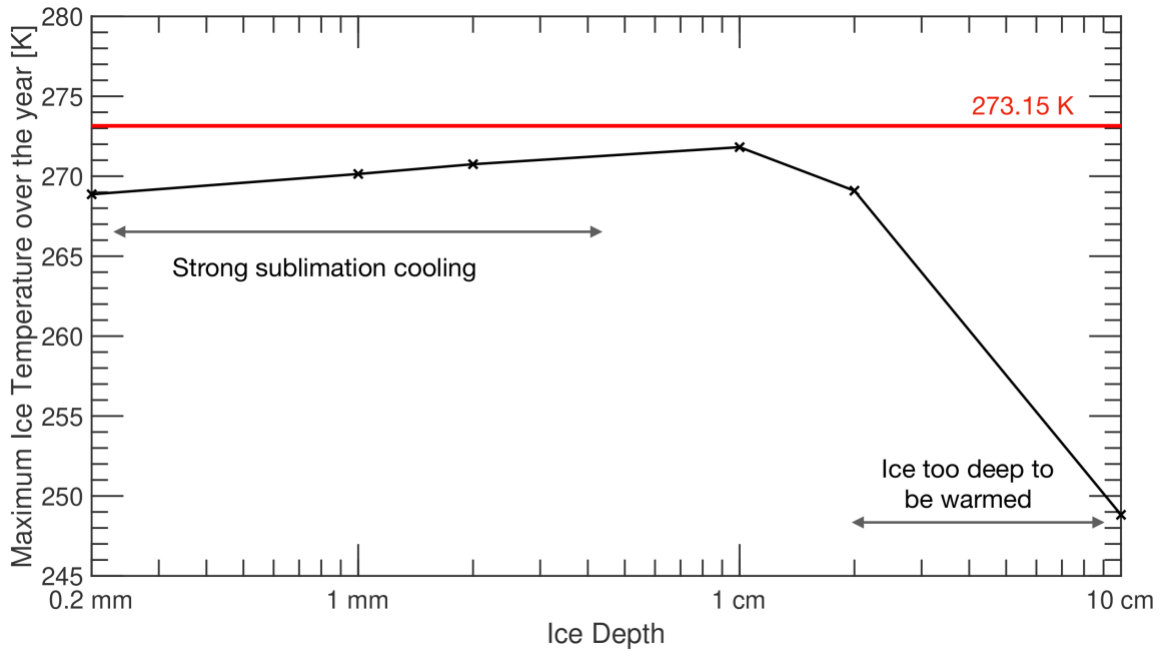

**Figure S3.** Maximum ice temperature as a function of the ice depth. Simulation is performed for a 30° pole-facing slope at 40°S, obliquity 35°, diffusion coefficient of  $10^{-5} \text{ m}^2 \text{ s}^{-1}$ , surface thermal inertia of  $350 \text{ J m}^{-2} \text{ K}^{-1} \text{ s}^{-1/2}$ , ice thermal inertia of  $800 \text{ J m}^{-2} \text{ K}^{-1} \text{ s}^{-1/2}$ .

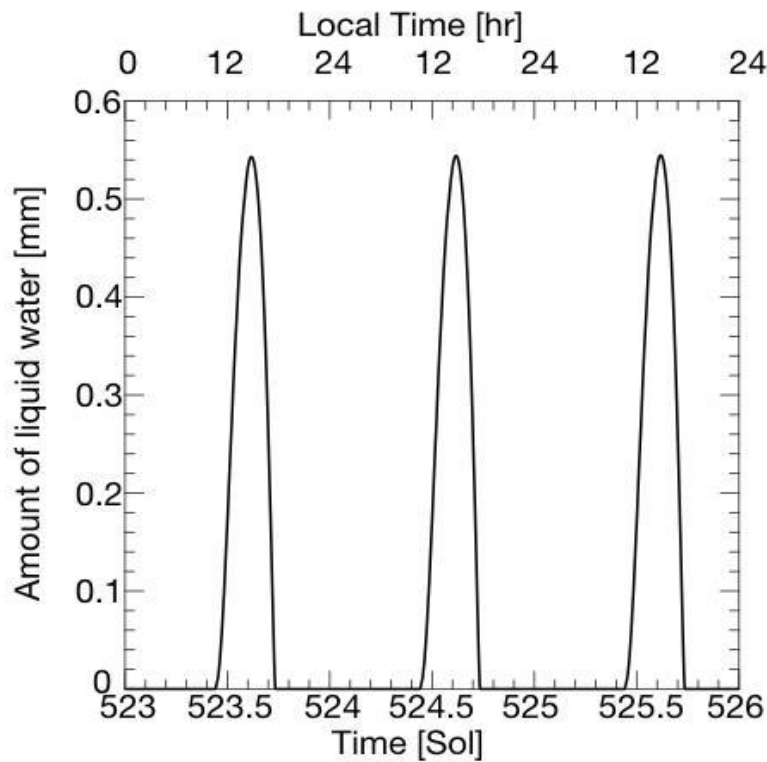

**Figure S4.** Amount of liquid water generated by the melting of ground ice after the removal of surface material. Simulation is performed at obliquity 35°, for a 30° pole-

facing slope at latitude 30°S, diffusion coefficient of  $10^{-5} \text{ m}^2 \text{ s}^{-1}$ , surface thermal inertia of  $350 \text{ J m}^{-2} \text{ K}^{-1} \text{ s}^{-1/2}$ , ice thermal inertia of  $800 \text{ J m}^{-2} \text{ K}^{-1} \text{ s}^{-1/2}$ . Ground ice is at a depth of 1 cm after being destabilized. Surface pressure is 1600 Pa. Solar longitude is  $\sim 276^\circ$ .

| Parameter                              | Value/Range of values                                                  |
|----------------------------------------|------------------------------------------------------------------------|
| Obliquity                              | 25.2°, 35°                                                             |
| Lsp                                    | 270°                                                                   |
| Eccentricity                           | 0.0934                                                                 |
| Latitude                               | 30°S, 40°S, 50°S                                                       |
| Slope angle                            | 0°-30°, 10° step, facing North and South                               |
| Subsurface ice initial depth $z_{ice}$ | 0.2 – 1 m                                                              |
| Albedo of bare ground                  | 0.13                                                                   |
| Thermal Inertia of dry soil            | 50 - 350 J m <sup>-2</sup> K <sup>-1</sup> s <sup>-1/2</sup>           |
| Thermal Inertia of water ice           | 800 – 1600 J m <sup>-2</sup> K <sup>-1</sup> s <sup>-1/2</sup>         |
| Surface Pressure (present-day)         | 400 - 800 Pa                                                           |
| Vapor in the column (present-day)      | 10 pr-μm                                                               |
| Surface Pressure (35° obliquity)       | 800-1600 Pa                                                            |
| Vapor in the column (35° obliquity)    | 260 pr-μm                                                              |
| Diffusion Coefficient                  | 4x10 <sup>-4</sup> , 1x10 <sup>-5</sup> m <sup>2</sup> s <sup>-1</sup> |
| Excavation factor α.                   | 0.9, 0.99, 0.999                                                       |

**Table S1.** Set-up for the simulations performed in section 3.3. Simulations are done in the South as it is where most of the gullies are observed.

## References:

- Clow, G. D., McKay, C. P., Simmons, G. M., & Wharton, R. A. (1988). Climatological Observations and Predicted Sublimation Rates at Lake Hoare, Antarctica. *Journal of Climate*, 1 (7), 715–728. doi:10.1175/1520-0442(1988)001<0715:coapsr>2.0.co;2
- Colaïtis, A., Spiga, A., Hourdin, F., Rio, C., Forget, F., & Millour, E. (2013). A thermal plume model for the Martian convective boundary layer. *Journal of Geophysical Research: Planets*, 118 (7), 1468-1487. doi: doi.org/10.1002/jgre.20104
- Douglas, T. A., & Mellon, M. T. (2019). Sublimation of terrestrial permafrost and the implications for ice-loss processes on Mars. *Nature Communications*, 10 (1). doi: 10.1038/s41467-019-09410-8
- England, D. E., & McNider, R. T. (1995). Stability functions based upon shear functions. *Boundary-Layer Meteorology*, 74 (1–2), 113–130. doi: 10.1007/bf00715713
- Fairall, C. W., Bradley, E. F., Rogers, D. P., Edson, J. B., & Young, G. S. (1996). Bulk parameterization of air-sea fluxes for Tropical Ocean-Global Atmosphere Coupled-Ocean Atmosphere Response Experiment. *Journal of Geophysical Research: Oceans*, 101 (C2), 3747–3764. doi: 10.1029/95jc03205
- Fairall, C. W., Bradley, E. F., Hare, J. E., Grachev, A. A., & Edson, J. B. (2003). Bulk Parameterization of Air–Sea Fluxes: Updates and Verification for the COARE Algorithm. *Journal of Climate*, 16 (4), 571–591. doi: 10.1175/1520-0442(2003)016<0571:bpoasf>2.0.co;2467
- Hébrard, E., Listowski, C., Coll, P., Marticorena, B., Bergametti, G., Mäattänen, A., . . . Forget, F. (2012). An aerodynamic roughness length map derived from extended Martian rock abundance data. *Journal of Geophysical Research (Planets)*, 117 (E4), E04008. doi: 10.1029/2011JE003942
- Khuller, A. R., & Clow, G. D. (2024). Turbulent Fluxes and Evaporation/Sublimation Rates on Earth, Mars, Titan, and Exoplanets. *Journal of Geophysical Research: Planets*, 129 (4). doi: 10.1029/2023je008114
- Lange, L., Piqueux, S., Edwards, C. S., Forget, F., Naar, J., Vos, E., & Szantai, A. (2024). Observations of Water Frost on Mars With THEMIS: Application to the Presence of Brines and the Stability of (Sub)Surface Water Ice. *Journal of Geophysical Research: Planets*, 129 (10). doi: 10.1029/2024je008489
- Schorghofer, N. (2020). Mars: Quantitative Evaluation of Crocus Melting behind Boulders. *The Astrophysical Journal*, 890 (1), 49. doi: 10.3847/1538-4357/ab612f
- Smith, M. D. (2002). The annual cycle of water vapor on Mars as observed by the Thermal Emission Spectrometer. *Journal of Geophysical Research: Planets*, 107 (E11), 25-1-25-19. doi: 10.1029/2001JE001522
